# Supplementary material for: Three-terminal Erasure Source-Broadcast with Feedback
Source: arXiv:2105.00353 source file (2021-05-01)
Supplement: Supplementary file 1 [file app.tex]

%\appendices
\section{Pseudocode for Algorithm of Section~\ref{subsec:instantly_decodable}}
\label{app:pseudocode}

\algdef{SE}[EVENT]{Event}{EndEvent}[1]{\textbf{upon event}\ #1\ \algorithmicdo}{\algorithmicend\ \textbf{event}}%
\algtext*{EndEvent}

\begin{algorithm}
\caption{Coding for Three Users with Feedback}\label{alg:three_users}
\begin{algorithmic}[1]
\State \textbf{Initialize}: $r_i \gets 0, \forall i \in \mathcal{U}$  % \Comment{Packets received by each user}
\ForAll {$t \in [N]$}
    \While {$\nexists \ i \in \mathcal{U} \ s.t.\ Z_i = 0$}
%    \State Send $S(t)$ until at least one user receives it
    	\State Transmit $S(t)$
    \EndWhile
%    \If {$\exists \ i \in \mathcal{U}, T \in \mathbb{N} \ s.t.\ N_i(T) = 0$}
%    \If {$\exists \ i \in \mathcal{U} \ s.t.\ N_i = 0$}
        \State $Q_{\mathcal{E}} \gets Q_{\mathcal{E}} \cup \{S(t)\}$
        \State $r_j\gets r_j + 1 \qquad \forall \ j \ s.t.\  Z_j = 0$
%    \EndIf
\EndFor

%\While{$\exists \ \textrm{distinct} i, j, k \in \mathcal{U}, i\neq j \neq k \ s.t.\ Q_i \neq \varnothing \ \textbf{and} \ \Q{j,k} \neq \varnothing$}
\While{$\exists \ \textrm{distinct} \ i, j, k \in \mathcal{U}, \ s.t.\ Q_i \neq \varnothing \ \textbf{and} \ \Q{j,k} \neq \varnothing$}
    \While {$\nexists \ l \in \mathcal{U} \ s.t.\ Z_l = 0$}
%	\State Let $q_i \in Q_i$, $q_{j,k} \in \Q{j,k}$ 
%       \State Transmit $q_i \oplus q_{j,k}$ until at least one user receives it  
       \State Transmit $q_i \oplus q_{j,k}$ where $q_i \in Q_i$, $q_{j,k} \in \Q{j,k}$ 
    \EndWhile
    \State $r_l\gets r_l + 1 \qquad \forall \ l \ s.t.\  Z_l = 0$
    \If {$Z_i = 0$}
    	\State $Q_i \gets Q_i \setminus \{q_i\}$
    \EndIf
    \If {$Z_j = 0 \ \textbf{and} \ Z_k = 1$}
    	\State $Q_k \gets Q_k \cup \{q_{j, k}\}$
       \State $\Q{j,k} \gets \Q{j, k} \setminus \{q_{j,k}\}$
    \ElsIf {$Z_j = 1 \ \textbf{and} \ Z_k = 0$}
    	\State $Q_j \gets Q_j \cup \{q_{j, k}\}$
	\State $\Q{j,k} \gets \Q{j, k} \setminus \{q_{j,k}\}$
    \ElsIf {$Z_j = 0 \ \textbf{and} \ Z_k = 0$}
    	\State $\Q{j,k} \gets \Q{j, k} \setminus \{q_{j,k}\}$
    \EndIf    
\EndWhile

\While{$Q_i \neq \varnothing \  \forall \ i \in \mathcal{U}$}
	\While {$\nexists \ l \in \mathcal{U} \ s.t.\ Z_l = 0$}
		\State Transmit $q_1 \oplus q_{2} \oplus q_{3}$, where $q_i \in Q_i \ \forall i \in \mathcal{U}$
	\EndWhile
	\ForAll {$l \in \mathcal{U} \ s.t.\ Z_l = 0$}
		\State $Q_l \gets Q_l \setminus \{q_l\}$
		\State $z_l \gets z_l + 1$
	\EndFor
\EndWhile

\Event{$ \exists \ i \ s.t.\ r_i \geq 1- d_i  $} %\Comment{One user finished}
%	\State Let $j, k \in \mathcal{U} \setminus \{i\}, \ s.t.\ j \neq k$
	\State $Q_j \gets Q_j \cup \Q{i,j} \qquad \forall \ j \in \mathcal{U} \setminus \{i\}$
	\State \textbf{run} two-user algorithm of Section~\ref{sec:two_users}
\EndEvent
\end{algorithmic}
\end{algorithm}
