# Supplementary material for: Three-terminal Erasure Source-Broadcast with Feedback
Source: arXiv:2105.00353 source file (2021-05-01)
Supplement: Supplementary file 5 [file chaining_newtheorem.tex]

%\newcommand{\rhoc}[2]{\ensuremath{\rhosub{c}(#1, #2)}}

%			$\rho_{i, l \to m}$ & Reward accumulated by user~$j$ after transition from state $l$ to $m$ \\
%			$\rho_{2, l \to m}$ &Reward accumulated by user~$k$ after transition from state $l$ to $m$ \\ 
%			$\rho_{c, l \to m}$ &Reward accumulated by user~$k$ after transition from state $l$ to $m$ \\ 
