# Supplementary material for: Three-terminal Erasure Source-Broadcast with Feedback
Source: arXiv:2105.00353 source file (2021-05-01)
Supplement: Supplementary file 6 [file markov_newtheorem.tex]

\newcommand{\chainsumOne}{\ensuremath{\sum_{k_1=1}^{\sizeS} \sum_{k_2 = 1}^{\sizeS} \ldots \sum_{k_{n-2} = 1}^{\sizeS}}}
\newcommand{\chainsum}{\ensuremath{\sum_{k_1=1}^{\sizeS} \sum_{k_2 = 1}^{\sizeS} \ldots \sum_{k_{n-1} = 1}^{\sizeS}}}

% States
%\newcommand{\sizeS}{\ensuremath{|\mathcal{S}|}}
\newcommand{\sizeS}{\ensuremath{|\myState|}}
\newcommand{\Si}[1]{\ensuremath{S_{#1}}}


% Transition Probabilities
\newcommand{\trans}[2]{\ensuremath{p_{#1#2}}}
\newcommand{\transM}{\ensuremath{P}}
\newcommand{\transMsup}[1]{\ensuremath{\transM^{#1}}}
\newcommand{\transMsupij}[3]{\ensuremath{\transMsup{#1}(#2, #3)}}
\newcommand{\transR}{\ensuremath{R}}
\newcommand{\transQ}{\ensuremath{Q}}

% Absorbing Markov Chains
\newcommand{\fundMat}{\ensuremath{N}}

% Reward Definitions
\newcommand{\rew}[2]{\ensuremath{\rho_{#1#2}}}
%\newcommand{\Rew}{\ensuremath{\Thorn}}
\newcommand{\Rew}{\ensuremath{\Theta}}
\newcommand{\RewSubAbsAbs}{\ensuremath{\Theta_{4}}}
\newcommand{\RewSubAbsTrans}{\ensuremath{\Theta_{3}}}
\newcommand{\RewSubTransAbs}{\ensuremath{\Theta_{2}}}
\newcommand{\RewSubTransTrans}{\ensuremath{\Theta_{1}}}

% Markov Chain submatricies
\newcommand{\RewSubCi}[1]{\ensuremath{B_{#1}}}
\newcommand{\RewSubDi}[1]{\ensuremath{A_{#1}}}
\newcommand{\RewSubC}{\ensuremath{\RewSubCi{n}}}
\newcommand{\RewSubD}{\ensuremath{\RewSubDi{n}}}

\newcommand{\HtransRew}{\ensuremath{H}}
\newcommand{\HSubAbsAbs}{\ensuremath{H_{4}}}
\newcommand{\HSubAbsTrans}{\ensuremath{H_{3}}}
\newcommand{\HSubTransAbs}{\ensuremath{H_{2}}}
\newcommand{\HSubTransTrans}{\ensuremath{H_{1}}}
\newcommand{\HtransRewij}[2]{\ensuremath{H(#1, #2)}}

% Expected Rewards
\newcommand{\Rni}[1]{\ensuremath{R_{#1}}}
\newcommand{\Rn}{\ensuremath{\Rni{n}}}
\newcommand{\Rnij}{\ensuremath{\Rn(i, j)}}

\newcommand{\barR}{\ensuremath{\bar{R}_{n}}}
\newcommand{\barRij}[2]{\ensuremath{\bar{R}_{n}(#1, #2)}}
\newcommand{\barRsubij}[3]{\ensuremath{\bar{R}_{#1}(#2, #3)}}
\newcommand{\barRinfij}[2]{\ensuremath{\barRsubij{\infty}{#1}{#2}}}
\newcommand{\barRinf}{\ensuremath{\bar{R}_{\infty}}}
\newcommand{\barRi}[1]{\ensuremath{\bar{R}_{n}(#1)}}
\newcommand{\barRinfi}[1]{\ensuremath{\barRi{#1}_{\infty}}}

\newcommand{\hatR}{\ensuremath{\hat{R}_{n}}}
\newcommand{\hatRij}[2]{\ensuremath{\hat{R}_{n}(#1, #2)}}


\newcommand{\hatRsub}[1]{\ensuremath{\hat{R}_{#1}}}
\newcommand{\hatRinf}{\ensuremath{\hatRsub{\infty}}}
\newcommand{\hatRsubij}[3]{\ensuremath{\hat{R}_{#1}(#2, #3)}}


% Markov Chain definitions
\newcommand{\myState}{\ensuremath{\Omega}}
\newcommand{\mystate}{\ensuremath{\Omega}}
\newcommand{\StateAbs}{\ensuremath{\myState_{A}}}
\newcommand{\StateTrans}{\ensuremath{\myState_{T}}}



%\newcommand{\bof}[1]{\textbf{#1}}
%\newcommand{\YN}[1]{\ensuremath{\tilde{Y}_{#1}^{n}}}
%\newcommand{\yN}[1]{\ensuremath{\tilde{y}_{#1}^{n}}}
%\newcommand{\tYN}[1]{\ensuremath{\tilde{Y}_{#1}^{n}}}
%\newcommand{\tyN}[1]{\ensuremath{\tilde{y}_{#1}^{n}}}
%\newcommand{\nN}[1]{\ensuremath{\tilde{n}_{#1}^{n}}}
%\newcommand{\NN}[1]{\ensuremath{\tilde{N}_{#1}^{n}}}
%\newcommand{\SHatK}[1]{\ensuremath{\hat{S}_{#1}^{m}}}
%%\newcommand{\setI}[1]{\ensuremath{\mathcal{I}(n_{#1}^{n})}}
%\newcommand{\setI}[1]{\ensuremath{I_{#1}}}
%\newcommand{\setInN}{\ensuremath{\mathcal{I}(n^n)}}
%\newcommand{\tSM}[1]{\ensuremath{\tilde{S}_{#1}^m}}
%\newcommand{\setURi}{\ensuremath{\mathcal{A}_i}}
%\newcommand{\setUR}{\ensuremath{\mathcal{A}}}
%\newcommand{\UN}{\ensuremath{U^n}}
%\newcommand{\uN}{\ensuremath{u^n}}
%\newcommand{\setIB}[1]{\ensuremath{\mathcal{I}_{#1}(u^n)}}
%\newcommand{\setIBH}[1]{\ensuremath{\mathcal{I}_{#1}(\hat{u}^n)}}
%\newcommand{\Prob}{\ensuremath{\operatorname{Pr}}}
%\newcommand{\Dstar}[1]{\ensuremath{D^{*}(\epsilon_{#1})}}
%%\newcommand{\XC}{\ensuremath{X_{\mathcal{\overline{C}(\nN{i})}}}}
%\newcommand{\oCn}{\ensuremath{\overline{\mathcal{C}}(\nN{i}, \nN{j})}}
%\newcommand{\Cn}{\ensuremath{\mathcal{C}(\nN{i}, \nN{j})}}
%\newcommand{\XC}{\ensuremath{X_{\oCn}}}
%\newcommand{\tUi}[1]{\ensuremath{\tilde{U}_{#1}}}
%\newcommand{\setV}{\ensuremath{\mathcal{V}}}
%\newcommand{\setU}{\ensuremath{\mathcal{U}}}
%\newcommand{\setA}{\ensuremath{\mathcal{A}}}
%\newcommand{\setB}{\ensuremath{\mathcal{B}}}
%\newcommand{\tUNn}{\ensuremath{\tilde{U}^n(\nS)}}
%\newcommand{\tUN}{\ensuremath{\tilde{U}^n}}
%
%\newcommand{\hpB}{\ensuremath{\hat{p}_{\setB}}}
%\newcommand{\pA}{\ensuremath{p_{\setA}}}
%\newcommand{\oCn}{\ensuremath{\overline{\mathcal{C}}(\nN{i}, \nN{j})}}
%\newcommand{\Cn}{\ensuremath{\mathcal{C}(\nN{i}, \nN{j})}}
%\newcommand{\XC}{\ensuremath{X_{\oCn}}}


\newcommand{\norm}[1]{\left\lVert#1\right\rVert}

%\newcommand{\YS}{\ensuremath{Y_{1}^n}}
%\newcommand{\YW}{\ensuremath{Y_{2}^n}}
%\newcommand{\NW}{\ensuremath{N_{2}^n}}
%\newcommand{\NS}{\ensuremath{N_{1}^n}}
%\newcommand{\nS}{\ensuremath{n_{1}^n}}
