# Supplementary material for: Three-terminal Erasure Source-Broadcast with Feedback
Source: arXiv:2105.00353 source file (2021-05-01)
Supplement: Supplementary file 7 [file one_sided_newtheorem.tex]

\newcommand{\nRepi}[1]{\ensuremath{M_{#1}}}
\newcommand{\vecnRep}{\ensuremath{\underline{M}}}
\newcommand{\indi}[1]{\ensuremath{\mathbbm{1}_{#1}}}

%\newcommand{\Nretransmit}{\ensuremath{\bar{N}_{0}}}
\newcommand{\Nretransmit}{\ensuremath{N_{0}}}
\newcommand{\ENretransmit}{\ensuremath{\mathbb{E}\Nretransmit}}

%\newcommand{\astar}{\ensuremath{\hat{a}}}
%\newcommand{\bstar}{\ensuremath{\hat{b}}}
\newcommand{\astar}{\ensuremath{c^{\dagger}}}
\newcommand{\bstar}{\ensuremath{d^{\dagger}}}
\newcommand{\cstar}{\ensuremath{a^{\dagger}}}
\newcommand{\mydstar}{\ensuremath{b^{\dagger}}}

\newcommand{\omegaparam}{\ensuremath{\theta}}
\newcommand{\gammaparam}{\ensuremath{\gamma}}

\newcommand{\omegastar}{\ensuremath{\omegaparam^{*}}}
\newcommand{\gammahat}{\ensuremath{\hat{\gammaparam}}}
\newcommand{\gammatilde}{\ensuremath{\gammaparam^{*}}}

\newcommand{\Fset}{\ensuremath{F}}
\newcommand{\Cset}{\ensuremath{C}}
\newcommand{\Aset}{\ensuremath{A}}
\newcommand{\AsetC}{\ensuremath{A^{\complement}}}
\newcommand{\Bset}{\ensuremath{B}}
\newcommand{\BsetOmega}{\ensuremath{B_{\omegaparam}}}
\newcommand{\BsetOmegaC}{\ensuremath{B_{\overline{\omegaparam}}}}
%\newcommand{\bOmegaC}{\ensuremath{b_{\overline{\omegaparam}}}}
\newcommand{\bOmegaC}{\ensuremath{b}}
\newcommand{\bOmegaPrime}{\ensuremath{b'}}
\newcommand{\bOmegaT}{\ensuremath{b_{\overline{\omegaparam}}(t)}}

\newcommand{\nFUnknown}{\ensuremath{N_{1}}}
\newcommand{\nBUnknown}{\ensuremath{N_{2}}}

\newcommand{\LHSfunc}{\ensuremath{\mathcal{L}}}
\newcommand{\LHSfuncparam}{\ensuremath{\LHSfunc(\gammaparam, \omegaparam)}}
\newcommand{\LHSfuncprime}{\ensuremath{\LHSfunc(\gammaparam', \omegaparam')}}

\newcommand{\kgamma}{\ensuremath{k_1}}
\newcommand{\komega}{\ensuremath{k_2}}
\newcommand{\kk}{\ensuremath{k_3}}

\newcommand{\wplusd}{\ensuremath{w^{+}(d_1, d_2)}}
\newcommand{\wid}{\ensuremath{w_{i}^{*}(d_i)}}
\newcommand{\wi}{\ensuremath{w_{i}^{*}}}
\newcommand{\wtwo}{\ensuremath{w_{2}^{*}(d_2)}}
\newcommand{\wone}{\ensuremath{w_{1}^{*}(d_1)}}

\newcommand{\depstwo}{\ensuremath{d_2/\epsilon_2}}
\newcommand{\depsone}{\ensuremath{d_1/\epsilon_1}}

\newcommand{\epsot}{\ensuremath{\epsilon_{12}}}

\newcommand{\donedagg}{\ensuremath{d_{1}^{\dagger}}}
\newcommand{\doneddagg}{\ensuremath{d_{1}^{\ddagger}}}

\newcommand{\donedaggall}{\ensuremath{\epsilon_1 (2\epsot - 1)/\epsot}}
\newcommand{\doneddaggall}{\ensuremath{\epsilon_1\epsot}}
